# Supplementary material for: Preserving Derivative Information while Transforming Neuronal Curves
Source: arXiv:2303.09649 source file (2023-08-01)
Supplement: Supplementary file 1 [file main-supplement.tex]

%%%%%%%%%%%%%%%%%%%%%%%%%%%%%%%%%%%%%%%%%%%%%%%%%%%%%%%%%%%%%%%%%%%%%
%%                                                                 %%
%% Please do not use \input{...} to include other tex files.       %%
%% Submit your LaTeX manuscript as one .tex document.              %%
%%                                                                 %%
%% All additional figures and files should be attached             %%
%% separately and not embedded in the \TeX\ document itself.       %%
%%                                                                 %%
%%%%%%%%%%%%%%%%%%%%%%%%%%%%%%%%%%%%%%%%%%%%%%%%%%%%%%%%%%%%%%%%%%%%%

%%\documentclass[referee,sn-basic]{sn-jnl}% referee option is meant for double line spacing

%%=======================================================%%
%% to print line numbers in the margin use lineno option %%
%%=======================================================%%

%%\documentclass[lineno,sn-basic]{sn-jnl}% Basic Springer Nature Reference Style/Chemistry Reference Style

%%======================================================%%
%% to compile with pdflatex/xelatex use pdflatex option %%
%%======================================================%%

%%\documentclass[pdflatex,sn-basic]{sn-jnl}% Basic Springer Nature Reference Style/Chemistry Reference Style

%%\documentclass[sn-basic]{sn-jnl}% Basic Springer Nature Reference Style/Chemistry Reference Style
\documentclass[pdflatex,sn-mathphys]{sn-jnl}% Math and Physical Sciences Reference Style

\usepackage{upgreek}

\newtheorem*{theorem*}{Theorem}

\jyear{2022}%

%% as per the requirement new theorem styles can be included as shown below
\theoremstyle{thmstyleone}%
%  meant for continuous numbers
%%\newtheorem{theorem}{Theorem}[section]% meant for sectionwise numbers
%% optional argument [theorem] produces theorem numbering sequence instead of independent numbers for Proposition
% 
%%\newtheorem{proposition}{Proposition}% to get separate numbers for theorem and proposition etc.

\theoremstyle{thmstyletwo}%

\theoremstyle{thmstylethree}%

\raggedbottom
%%\unnumbered% uncomment this for unnumbered level heads

\begin{document}
\title[Supplement: Preserving...Information while Transforming Neuronal Curves]{Supplement: Preserving Higher Order Information while Transforming Neuronal Curves}
    
    \author*[1,2]{\fnm{Thomas L.} \sur{Athey}}\email{tathey1@jhu.edu}
    
    \author[3,4]{\fnm{Daniel J.} \sur{Tward}}\email{DTward@mednet.ucla.edu}
    
    \author[5]{\fnm{Ulrich} \sur{Mueller}}\email{umuelle3@jhmi.edu}

    \author[2,6,7,8]{\fnm{Laurent} \sur{Younes}}\email{laurent.younes@jhu.edu}
    \author[1,2,7,8]{\fnm{Michael I.} \sur{Miller}}\email{mim@cis.jhu.edu}

    \affil*[1]{\orgdiv{Department of Biomedical Engineering}, \orgname{Johns Hopkins University}, \orgaddress{\city{Baltimore}, \state{MD}, \country{USA}}}

    \affil[2]{\orgdiv{Institute of Computational Medicine}, \orgname{Johns Hopkins University}, \orgaddress{\city{Baltimore}, \state{MD}, \country{USA}}}
    
    \affil[3]{\orgdiv{Department of Computational Medicine}, \orgname{University of California at Los Angeles}, \orgaddress{ \city{Los Angeles}, \state{CA}, \country{USA}}}
    
    \affil[4]{\orgdiv{Department of Neurology}, \orgname{University of California at Los Angeles}, \orgaddress{ \city{Los Angeles}, \state{CA}, \country{USA}}}
    
    \affil[5]{\orgdiv{Department of Neuroscience}, \orgname{Johns Hopkins University}, \orgaddress{\city{Baltimore}, \state{MD}, \country{USA}}}
    
    \affil[6]{\orgdiv{Department of Applied Mathematics \& Statistics}, \orgname{Johns Hopkins University}, \orgaddress{\city{Baltimore}, \state{MD}, \country{USA}}}
    
    \affil[7]{\orgdiv{Center for Imaging Science}, \orgname{Johns Hopkins University}, \orgaddress{\city{Baltimore}, \state{MD}, \country{USA}}}
    
    \affil[8]{\orgdiv{Kavli Neuroscience Discovery Institute}, \orgname{Johns Hopkins University}, \orgaddress{\city{Baltimore}, \state{MD}, \country{USA}}}

\maketitle

\input{nature_methods_brief_comm/supplement}

\bibliography{refs}
\end{document}
